# Supplementary material for: A time-adaptive finite element phase-field model suitable for rate-independent fracture mechanics
Source: arXiv:2403.07461 source file (2024-03-12)
Supplement: Supplementary file 1 [file Appendix.tex]

\section{Implementation of norms}
 \label{Appendix_1}
The for the implementation of the $L_p$-norm relevant quantities are 
\begin{flalign}
g=\norm{z-z_{j-1}}_{L_p}-\rho=\bigg[\underset{=:\Sint}{\underbrace{\int_{\Omega}[z-z_{j-1}]^p\dd{V}}}\bigg]^{\frac{1}{p}}-\rho\\
b=\frac{1}{p^2}\left[(1-p)\Sint^{\frac{1-2p}{p}}\max\left\{0,\lambda_2+\alpha_2 g\right\}+\alpha_2\Sint^{\frac{2-2p}{p}}H(\lambda_2+\alpha_2g)\right]\\
\boldsymbol{\mathrm{f}}_z^{e,A}=p\int_{\Omega_e}N_A (z-z_{j-1})^{p-1}\dd{V}\\
%\boldsymbol{\mathrm f}_{z,EM}^{e,A}=\max\left\{0,\lambda_2+\alpha_2g\right\}\Sint^{\frac{1-p}{p}}\int_{\Omega_e}N_A(z-z_{j-1})^{p-1}\dd{V}\\
\boldsymbol{\mathrm K}_{sp,EM}^{e,AB}=[p-1]\max\left\{0,\lambda_2+\alpha_2g\right\}\Sint^{\frac{1-p}{p}}\int_{\Omega_e}N_A N_B [z-z_{j-1}]^{p-2}\dd{V}.
\end{flalign}
The terms for the $H_1$-norm are
\begin{flalign}
g=\norm{z-z_{j-1}}_{H_1}-\rho=\bigg[\underset{=:\Sint}{\underbrace{\int_{\Omega}[z-z_{j-1}]^2+|\gradx(z-z_{j-1})|^2\dd{V}}}\bigg]^{\frac{1}{2}}-\rho\\
b=\frac{1}{4}\left[\Sint^{\frac{-3}{2}}\max\left\{0,\lambda_2+\alpha_2 g\right\}+\alpha_2 \Sint^{-1}H(\lambda_2+\alpha_2g)\right]\\
\boldsymbol{\mathrm{f}}_z^{e,A}=2\int_{\Omega_e}N_A [z-z_{j-1}]+\gradx(z-z_{j-1})\cdot \BA\dd{V}\\
%\boldsymbol{\mathrm f}_{z,EM}^{e,A}=\max\left\{0,\lambda_2+\alpha_2g\right\}\Sint^{-\frac{1}{2}}\int_{\Omega_e}N_A(z-z_{j-1})+\gradx (z-z_{j-1})\cdot \BA\dd{V}\\
\boldsymbol{\mathrm K}_{sp,EM}^{e,AB}=\max\left\{0,\lambda_2+\alpha_2g\right\}\Sint^{-\frac{1}{2}}\int_{\Omega_e}N_A N_B + \BA\cdot\BB \dd{V}
\end{flalign}
%The terms for the $\calG_f$-norm follow in the same manner as
%\begin{flalign}
%g=\underset{=:\Sint}{\underbrace{\frac{g_c}{2}\int_{\Omega}\frac{[1-z]^2-[1-z_{j-1}]^2}{l}+l\left[\norm{\gradx z}^2-\norm{\gradx z_{j-1}}^2\right]\dd{V}}}-\rho\\
%b=\alpha_2 H(\lambda_2+\alpha_2g)\\
%\boldsymbol{\mathrm{f}}_z^{e,A}=\frac{g_c}{l}\int_{\Omega_e}N_A [z-1]+l^2\gradx z \cdot \BA\dd{V}\\
%%\boldsymbol{\mathrm f}_{z,EM}^{e,A}=\max\left\{0,\lambda_2+\alpha_2g\right\}\frac{g_c}{l}\int_{\Omega_e}N_A (z-1)+l^2\gradx z \cdot \BA\dd{V}\\
%\boldsymbol{\mathrm K}_{sp,EM}^{e,AB}=\max\left\{0,\lambda_2+\alpha_2g\right\}\frac{g_c}{l}\int_{\Omega_e}N_A N_B + l^2\BA\cdot\BB \dd{V}
%\end{flalign}
